# Supplementary material for: Physics-Based Simulation of Contact-Induced Facial Wrinkling
Source: arXiv:2607.04768 source file (2026-07-06)
Supplement: Supplementary file 1 [file Appendix.tex]

\appendix

%\section{Plasticity Model}
\section{Material Modeling}
